# Supplementary material for: Rayleigh-Taylor instability under an inclined plane
Source: arXiv:1503.02345 ancillary file (2015-03-08)
Supplement: Supplementary file 1 [file suppl1.pdf]

# Supplemental material for Rayleigh Taylor instability under an inclined plane

P.-T. Brun, Adam Damiano, Pierre Rieu, Gioele Balestra, François Gallaire

March 8, 2015

We detail the method used to define the area of interest and determine the number of droplets dripping in this region over the course of our experiments. The analysis is conducted on the movies captured by the camera positioned in the experimental setup as described in the main text (Fig. 1). It combines an image processing software (ImageJ) to a symbolic software (Mathematica in the present case).

## 1 Data gathering: thin film contour and droplets

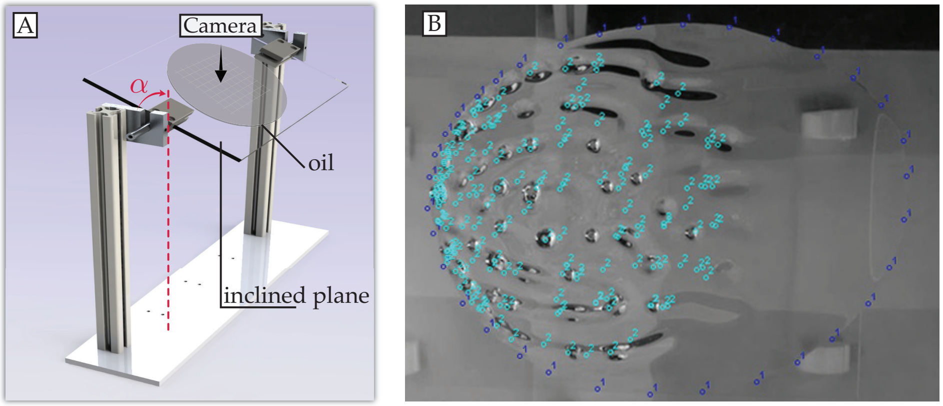


Figure 1: A: The experimental setup. B: A discrete set of data points defines the the film perimeter (label 1) and the dripping positions (label 2)

The first step consists in delimiting the film perimeter position with a set of points denoted $\mathbf{x}_i$, typically 50. They are positioned on contact line

between the fluid and the surface on the first frame captured after the initial rotation of the surface. Second, the movie is played frame by frame and the dripping positions of each drop $\mathbf{y}_i$ are captured manually along with the corresponding dripping time. A typical result is shown in Fig. 1.

## 2 Data analysis

The area of interest is obtained by scaling the film perimeter inwards in order to discard the droplets forming by interaction with the contact line and focus on the central area of the film. Discrete differentiation of the film contour points $\mathbf{x}_i$ yields a set of normals to the perimeter, $\mathbf{n}_i$, pointing inward. A new set of points, $\bar{\mathbf{x}}_i$, is derived by translation of each point $\mathbf{x}_i$ on a length $\delta$ along the vectors $\mathbf{n}_i$ (see Fig. 2). We used $\delta = 2\lambda$, where $\lambda = 2\pi\sqrt{2}\ell_c$ is the typical size of a droplet. Finally, the number of the droplets $\mathbf{y_i}$ lying in the area of interest $\bar{\mathbf{x}}_i$ is evaluated following a conventional point-in-polygon algorithm[1].

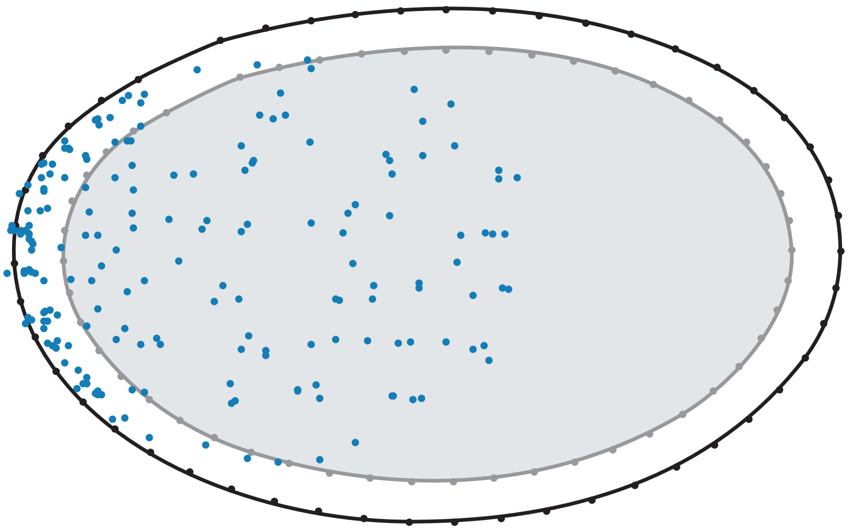

Figure 2: Outer contour of the thin film (black), area of interest (gray) and drops positions (blue points): 79 droplets are found in the area of interest

[1] see for example http://demonstrations.wolfram.com/AnEfficientTestForAPointToBeInAConvexPolygon/ for an example
